# Supplementary material for: Excitation Pathways in Resonant Inelastic X-Ray Scattering of Solids
Source: arXiv:2002.12876 source file (2020-02-28)
Supplement: Supplementary file 1 [file supplementary-information.pdf]

# Supplementary Information: Excitation Pathways in Resonant Inelastic X-Ray Scattering of Solids

Christian Vorwerk,[1,2,*] Francesco Sottile,[3,4] and Claudia Draxl[1,4]

[1] *Physics Department and IRIS Adlershof, Humboldt-Universität zu Berlin, Berlin, Germany*
[2] *European Theoretical Spectroscopy Facility (ETSF)*
[3] *LSI, Ecole Polytechnique, CNRS, CEA, Institut Polytechnique de Paris, F-91128 Palaiseau, France*
[4] *European Theoretical Spectroscopic Facility (ETSF)*

(Dated: February 28, 2020)

## NOVEL EXPRESSION FOR THE RIXS CROSS SECTION

The *double-differential cross section* (DDCS) yields the probability to scatter an incident x-ray photon with energy $\omega$ and polarization $\mathbf{e}_1$, such that an x-ray photon with energy $\omega'$ and polarization $\mathbf{e}_2$ is emitted, with a momentum loss into a solid angle $d\Omega$. The DDCS of the RIXS process is given by the Kramers-Heisenberg formula [1] as

$$\frac{\mathrm{d}^2\sigma}{\mathrm{d}\Omega \mathrm{d}\omega'} \propto \sum_F \left| \sum_I \frac{\langle F|\hat{D}^\dagger(\mathbf{e}_2)|I\rangle\langle I|\hat{D}(\mathbf{e}_1)|0\rangle}{\omega - E_I + \mathrm{i}\eta_I} \right|^2 \times \times \delta((E_F - E_0) + \omega' - \omega), \tag{1}$$

where $|0\rangle$, $|I\rangle$, $|F\rangle$ denote the many-body ground state, intermediate state, and final state with energies $E_0$, $E_I$, and $E_F$, respectively. $\hat{D}(\mathbf{e}_1) = \sum_j \mathbf{e}_1 \cdot \mathbf{p}_j$ denotes the many-body dipole operator. Here, we ignore the first order scattering term, which yields the non-resonant inelastic x-ray scattering (NIXS). The NIXS term has been investigated within the many-body formalism. Ample literature is available both for the vanishing [2, 3] and finite momentum transfer NIXS [4–6]. We now express the transition operator in second quantization by introducing an arbitrary single-particle basis $\{\phi_{i\mathbf{k}}\}$ with its corresponding particle creation $\hat{c}^\dagger_{i\mathbf{k}}$ and annihilation operators $\hat{c}_{i\mathbf{k}}$. This leads to the expression $\hat{D}(\mathbf{e}) = \sum_{ij\mathbf{k}} d_{ij\mathbf{k}} \hat{c}^\dagger_{j\mathbf{k}} \hat{c}_{i\mathbf{k}}$ with $d_{ij\mathbf{k}} = \langle i\mathbf{k}|\mathbf{e}\cdot\mathbf{p}|j\mathbf{k}\rangle$. We furthermore employ the Lehman representation (with generic excited many-body states $|n\rangle$) of the polarizability $\chi$ using occupied orbitals $\phi_{j\mathbf{k}}$ and conduction orbitals $\phi_{i\mathbf{k}}$ as

$$\chi_{ij\mathbf{k},i'j'\mathbf{k}'}(\omega) = \sum_{n\neq 0} \frac{\langle 0|\hat{c}^\dagger_{j\mathbf{k}}\hat{c}_{i\mathbf{k}}|n\rangle\langle n|\hat{c}^\dagger_{i'\mathbf{k}'}\hat{c}_{j'\mathbf{k}'}|0\rangle}{\omega - (E_n - E_0) + \mathrm{i}\eta}. \tag{2}$$

We consider semiconducting and insulating systems, for which the distinction between occupied and unoccupied states is unambiguous. The full polarizability can be easily generalized even to metal systems, using fractional occupation numbers, following Fermi statistics. This is, however, not our target, since excitonic effects vanish in metallic systems. Using this representation, we can express the DDCS as

$$\frac{\mathrm{d}^2\sigma}{\mathrm{d}\Omega \mathrm{d}\omega'} \propto \mathrm{Im} \sum_{\substack{c,c',c'',c''' \\ v,v' \\ \mu,\mu',\mu'',\mu'''}} \sum_{\substack{\mathbf{k},\mathbf{k}' \\ \mathbf{k}'',\mathbf{k}'''}} \left[d'_{\mu v\mathbf{k}} \chi_{c\mu\mathbf{k},c'\mu'\mathbf{k}'}(\omega) d_{c'\mu'\mathbf{k}'}\right]^* \times \times \chi_{cv\mathbf{k},c''v'\mathbf{k}''}(\omega-\omega') \times \times \left[d'_{\mu''v'\mathbf{k}''} \chi_{c''\mu''\mathbf{k}'',c'''\mu'''\mathbf{k}'''}(\omega) d_{c'''\mu'''\mathbf{k}'''}\right]. \tag{3}$$

Here, the summation includes core states $\mu, \mu', \mu'', \mu'''$, valence states $v, v'$, and conduction states $c, c', c'', c'''$. Note that we evaluate the polarizability $\chi$ in the basis of core and conduction states at the incoming x-ray frequency $\omega$, and in the basis of valence and conduction states at the energy loss $\omega - \omega'$. The polarizability is obtained in many-body perturbation theory from the solutions of the Bethe-Salpeter equation

$$\begin{aligned}\chi_{cv\mathbf{k},c'v'\mathbf{k}'}(\omega) &= \left[\chi_0^{-1}(\omega) - \Xi\right]^{-1}_{cv\mathbf{k},c'v'\mathbf{k}'} \\ &= -\left[H^{BSE} - \omega\right]^{-1}_{cv\mathbf{k},c'v'\mathbf{k}'},\end{aligned} \tag{4}$$

where the non-interacting polarizability is given by

$$\chi_0 = \frac{\delta_{vv'}\delta_{cc'}\delta_{\mathbf{k}\mathbf{k}'}}{\omega - (\epsilon_{c\mathbf{k}} - \epsilon_{v\mathbf{k}}) + i\eta}, \tag{5}$$

and is thus diagonal in this space. The interaction kernel $\Xi = v + W$. The Coulomb interaction $v = \frac{1}{|\mathbf{r}-\mathbf{r}'|}$ and the statically screened interaction $W = \varepsilon^{-1}v$ constitute the ingredients of BSE, as it is nowadays found in many implementations. In the second line of Eq. 4, all frequency-independent terms are included in the BSE Hamiltonian $H^{BSE}$. The eigenvalues $E^\lambda$ and corresponding eigenstates $A_{ij\mathbf{k},\lambda}$ of $H^{BSE}A_\lambda = E^\lambda A_\lambda$ yield the polarizability as

$$\chi_{cv\mathbf{k},c'v'\mathbf{k}'}(\omega) = -\sum_\lambda \frac{A_{cv\mathbf{k},\lambda}\left[A_{c'v'\mathbf{k}',\lambda}\right]^*}{E^\lambda - \omega - \mathrm{i}\eta}. \tag{6}$$

Here, we employ the so-called Tamm-Dancoff approximation, *i.e.* we neglect the coupling of resonant and anti-resonant excitations in the BSE Hamiltonian. We note that if the polarizability $\chi^0_{vc,v'c'}$ in the independent-particle approximation (IPA) is inserted in the double-differential cross section, we recover the well-known independent-particle RIXS cross section [7, 8].

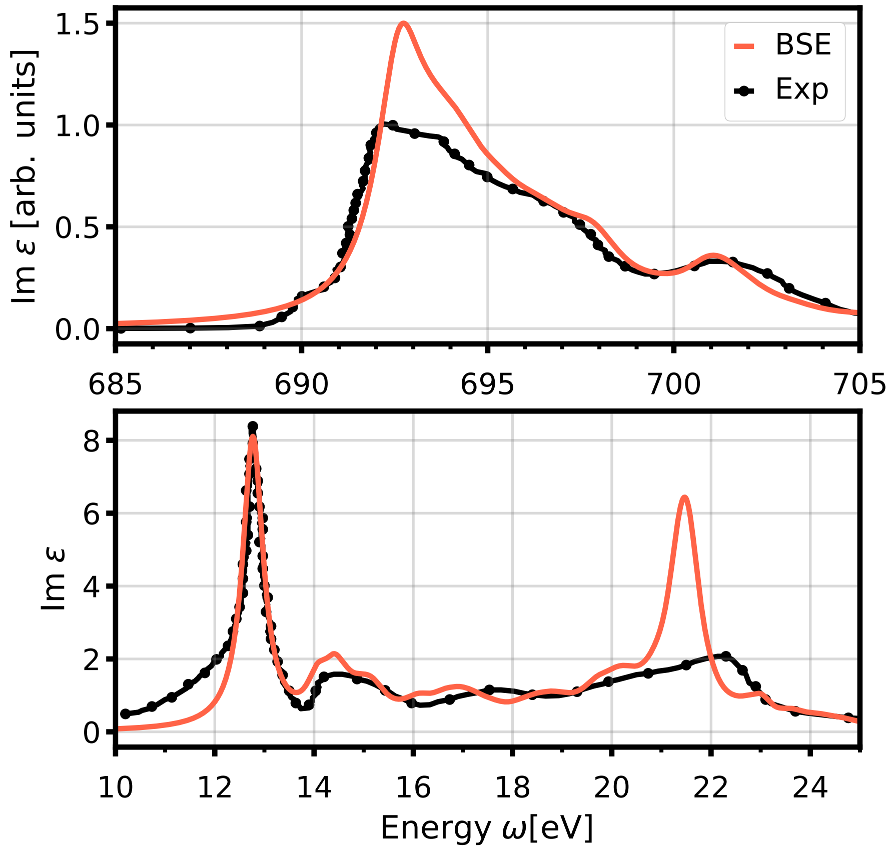


FIG. 1. F K edge absorption spectrum (top) and optical absorption spectrum (bottom) of LiF. The calculated spectra are shown in red, the experimental spectra in black. The experimental optical spectrum is obtained from Ref. [9], the experimental F K edge spectrum from Ref. [10].

## COMPUTATIONAL DETAILS

All calculations are perfomed using the all-electron full-potential code `exciting` [6, 11, 12]. The electronic ground state of LiF is calculated on an $8 \times 8 \times 8$ **k**-grid. We include basis functions up to a cut-off off $R_{MT,max} \cdot |\mathbf{G}+\mathbf{k}|_{max} = 9.0$. The muffin-tin (MT) spheres are set to a radius $R_{MT}(Li) = 2.10\ a_0$ and $R_{MT}(F) = 1.70\ a_0$ for all calculations. For all calculations, we employ the generalized gradient approximation to the exchange-correlation functional as proposed in Ref. [13]. Both the optical and the F K edge absorption spectra are calculated on a $9 \times 9 \times 9$ **k**-grid, which is shifted by $\Delta\mathbf{k} = (0.05, 0.15, 0.25)^T$. Local field effects are included up to a cut-off $|\mathbf{G}+\mathbf{q}|_{\max} = 7.0\ a_0^{-1}$. The screened Coulomb interaction is calculated in the random-phase approximation (RPA) including all valence and 100 empty states. For the optical absorption spectrum, the BSE Hamiltonian is constructed from the 4 valence states and the lowest 20 unoccupied states, which yields a transition space of $9^3 \cdot 4 \cdot 20 = 58320$ transitions. For the F K edge spectrum, the Hamiltonian is constructed from the F 1$s$ states and the lowest 20 unoccupied states, resulting in a transition space of 29610 transitions. The calculated absorption spectra are shown in Fig. 1 compared to experimental results for the optical [9] and F K edge spectra [10]. A Lorentzian lifetime broadening of 0.75 eV for the F K edge spectrum and 0.25 eV for the optical spectrum is employed. The increased broadening for the F K edge spectrum reflects the shorter lifetime of the F 1$s$ state. A scissors shift of 5.873 eV is applied to the calculated optical spectrum to account for the underestimation of the band gap in the DFT electronic structure. For the F K edge spectrum, a scissors operator of 36 eV is applied, which accounts both for the underestimated band gap and the underestimation of the F 1$s$ binding energy in the DFT calculation.

The RIXS spectrum is constructed from the lowest 12000 optical BSE eigenvectors, which yields an energy loss of up to 35 eV, and the lowest 6000 core BSE eigenvectors, which allows for the calculation of spectra at excitation energies of up to 706 eV. A Lorentzian broadening of 0.15 eV is applied to the core-excited intermediate state and the final valence-excited one. Experimental

RIXS spectra are reported in Ref. [14] in arbitrary units. In order to compare experimental and calculated spectra, we normalize the calculated RIXS DDCS at each excitation energy, such that the calculated and experimental maximum agree.

## FLUORESCENCE FOR EXCITATIONS BELOW THE ABSORPTION ONSET

In main text, we report the F K edge RIXS spectra for excitation energies beyond the F K edge onset at 691.8 eV. Experimental spectra are also available below the onset, and we report the calculated spectra in Fig. 2. In this excitation region, the calculated BSE spectra disagree qualitatively from the experimental ones: A strong peak at emission energies of approximately 677.3 eV is completely missing in our calculations, which predicts that emission only occurs at considerably higher energy loss, *i.e.* lower emission energies. For excitations in this energy region, no core excitation is excited resonantly, and the spectrum is formed by the life-time tails of many excitations over a wide energy range. In our calculations, the loss occurs predominantely at 14 eV, independently of the excitation energy yielding the broad emission feature in Fig. 2. The presence of a linearly dispersive broad absorption feature, *i.e.* features at constant energy loss, in the sub-threshold RIXS spectrum have been observed for LiF [14], Cu, and Ni [15] before. These features occur,since no core excitation is in resonance with the incoming x-ray energy, and as such no core excitation is strongly favored over the others. As a result, the emission spectrum does not strongly depend on the absorption energy and thus reflects the shape of the optical absorption spectrum. The experimental spectra, on the other hand, shows an additional peak at approximately 677.4 eV for all excitation energies below the onset. With increasing excitation energy, the peak becomes more dominant until, at 689.8 eV, it dominates the experimental spectrum.

If we consider the excitation at 688 eV, the initial peak at 677.4 corresponds to an energy loss of around 10.6 eV, well below the onset of absorption in the optical spectra (see lower panel in Fig. 1). This indicates that the emission does not originate from the absorption of a x-ray photon with an energy of 688.0 eV, but rather of a photon with higher energy, such that the energy loss is actually higher. This can occur if the incoming x-ray beam is not perfectly monochromatic, but rather has a finite linewidth [14, 16]. For a given excitation energy, we then have to consider the scattering of x-ray photons within a range of energies around the given excitation energy. Following Ref. [14], we express the double-differential cross section as a function of the excitation energy $\omega$ and emis-

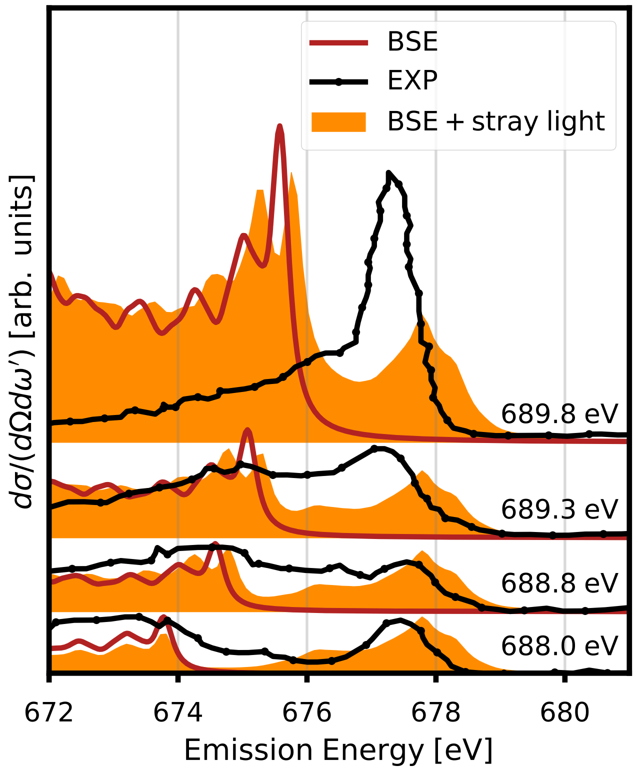


FIG. 2. F K edge RIXS spectrum calculated from BSE (red) and from BSE including stray-light contributions (orange) and from experiment (black) [14]. The calculated spectra are normalized to the experimental ones for each excitation energy. A lifetime broadening of 0.15 eV is employed for all calculated spectra. The parameter of the stray-light contribution are described in the text.

sion energy $\omega'$ and obtain

$$\frac{\mathrm{d}\sigma}{\mathrm{d}\Omega\mathrm{d}\omega'}(\omega,\omega') = \int d\omega'' \frac{\mathrm{d}\sigma}{\mathrm{d}\Omega\mathrm{d}\omega'}\bigg|_{\mathrm{BSE}}(\omega'',\omega')\cdot\eta(\omega''-\omega'), \tag{7}$$

where $\frac{\mathrm{d}\sigma}{\mathrm{d}\Omega\mathrm{d}\omega'}\Big|_{\mathrm{BSE}}(\omega,\omega')$ is the DDCS calculated from BSE for a given excitation energy $\omega''$, while $\eta(\omega''-\omega')$ describes the linewidth of the excitation energy. In the derivation of the DDCS, we assume $\eta(\omega''-\omega')\to\delta(\omega''-\omega')$. Now, we assume that there is an additional Lorentzian background with a width $\Delta$ and a relative intensity $\xi$, such that

$$\eta(\omega''-\omega') = \delta(\omega''-\omega') + \xi\frac{\Delta^2}{\Delta^2+(\omega''-\omega')^2}. \tag{8}$$

The second term is called the *stray-light contribution*. In Fig. 2, we add stray-light corrections using a distribution of $\Delta$= 20 eV and $\xi$ = 0.001 in agreement with the parameters of Ref. [14]. The stray-light contribution correctly introduces the peak at high emission energies, but our calculations yield a peak at slightly overestimated

emission energies. Our analysis shows that the peak originates from the strong RIXS signal that occurs at an excitation energy of 692 eV and an energy loss of 14 eV (see Fig. 2 in the Letter). Due to the linewidth of the excitation energy, even at considerably lower excitation energies below the absorption onset, some initial x-ray photons have an energy of 692 eV and are scattered such that the emitted photon has an energy of 678 eV. Due to the low signal of the scattering rate for x-ray photons with energies below the absorption onset, the peak at 678 eV is strong. We find that the agreement is better at lower excitation energies than at 689.8 eV. The linewidth of the excitation energy $\eta(\omega''-\omega')$ depends on the set-up of the measurement, and at higher excitation energies it deviates from Lorentzian shape.

* vorwerk@physik.hu-berlin.de

[1] H. A. Kramers and W. Heisenberg, Z. Phys. **31**, 681 (1925).
[2] V. Olevano and L. Reining, Phys. Rev. Lett. **86**, 5962 (2001).
[3] G. Onida, L. Reining, and A. Rubio, Rev. Mod. Phys. **74**, 601 (2002).
[4] M. Gatti and F. Sottile, Phys. Rev. B **88**, 155113 (2013).
[5] J. Koskelo et al., Phys. Rev. B **95**, 035125 (2017).
[6] C. Vorwerk, B. Aurich, C. Cocchi, and C. Draxl, Electronic Structure **1**, 037001 (2019).
[7] Y. Ma et al., Phys. Rev. Lett. **69**, 2598 (1992).
[8] P. D. Johnson and Y. Ma, Phys. Rev. B **49**, 5024 (1994).
[9] K. K. Rao, T. J. Moravec, J. C. Rife, and R. N. Dexter, Phys. Rev. B **12**, 5937 (1975).
[10] Y. Joly, C. Cavallari, S. A. Guda, and C. J. Sahle, Journal of Chemical Theory and Computation **13**, 2172 (2017).
[11] A. Gulans et al., J. Phys. Condens. Matter. **26**, 363202 (2014).
[12] C. Vorwerk, C. Cocchi, and C. Draxl, Phys. Rev. B **95**, 155121 (2017).
[13] J. P. Perdew et al., Physical Review Letters **100**, 136406 (2008).
[14] A. Kikas et al., Phys. Rev. B **70**, 085102 (2004).
[15] M. Magnuson et al., Phys. Rev. B **68**, 045119 (2003).
[16] R. Feifel et al., Journal of Electron Spectroscopy and Related Phenomena **134**, 49 (2004).
